# Supplementary material for: Role of ALD Al2O3 surface passivation on the performance of p-type Cu2O thin film transistors
Source: arXiv:2010.10928 source file (2020-10-21)
Supplement: Supplementary file 1 [file Supprorting_information.pdf]

# Supporting Information

## Role of ALD $Al_2O_3$ surface passivation on the performance of p-type $Cu_2O$ thin film transistors

M Napari[1*], T N Huq[1], D J Meeth[2], M J Heikkilä[3], K M Niang[2], Han Wang[4] ,T Iivonen[3†], Haiyan Wang[4], M Leskelä[3], M Ritala[3], A J Flewitt[2], R L Z Hoye[1‡] J L MacManus-Driscoll[1]

[1] *Department of Materials Science and Metallurgy, University of Cambridge, UK*

[2] *Electrical Engineering Division, Department of Engineering, University of Cambridge, UK*

[3] *Department of Chemistry, University of Helsinki, FIN*

[4] *Materials Engineering, Purdue University, US*

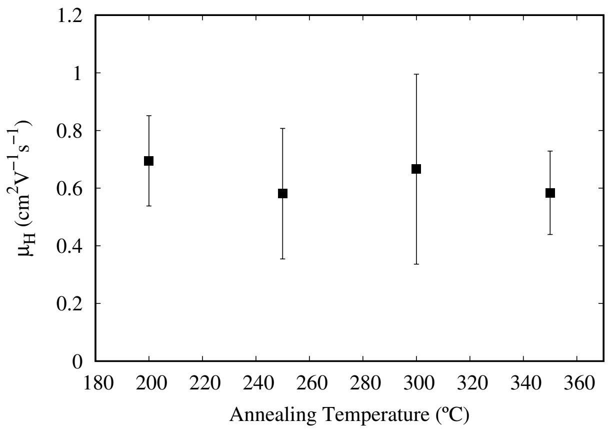


Figure S1: Hall-measured hole mobility $\mu_H$ in the annealed $Cu_2O$ films. Data point at 200 °C represents the as-deposited film. The errorbars are the standard deviation of the multiple measurements taken from two samples annealed in same conditions.

*Present address: Zepler institute for Photonics and Nanoelectronics, University of Southampton, Southampton, UK
†Present address: Nanoform Finland Oyj, Helsinki, FIN
‡Present address: Department of Materials, Imperial College London, UK

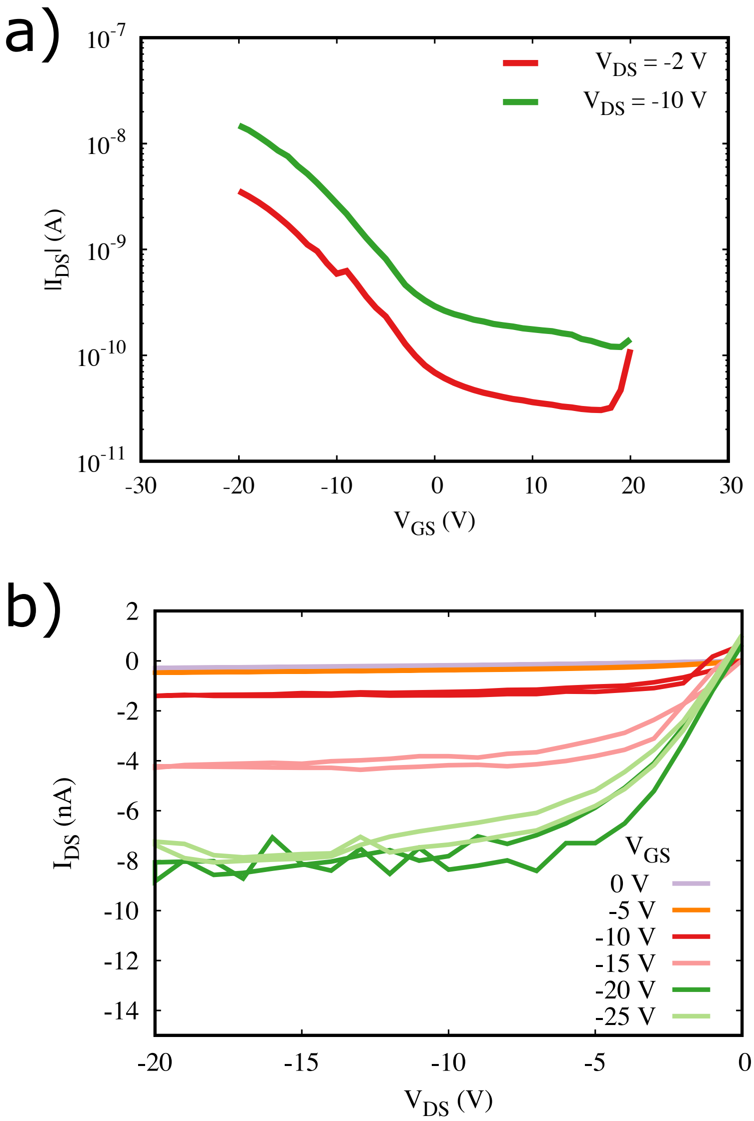


Figure S2: a) Transfer characteristics of a $Cu_2O$ p-channel TFT with 75 nm $Al_2O_3$ gate oxide, the device is passivated with 10 nm $Al_2O_3$ and subsequently annealed at 300 °C, W/L = 20. (b) TFT output characteristics measured from the same device.

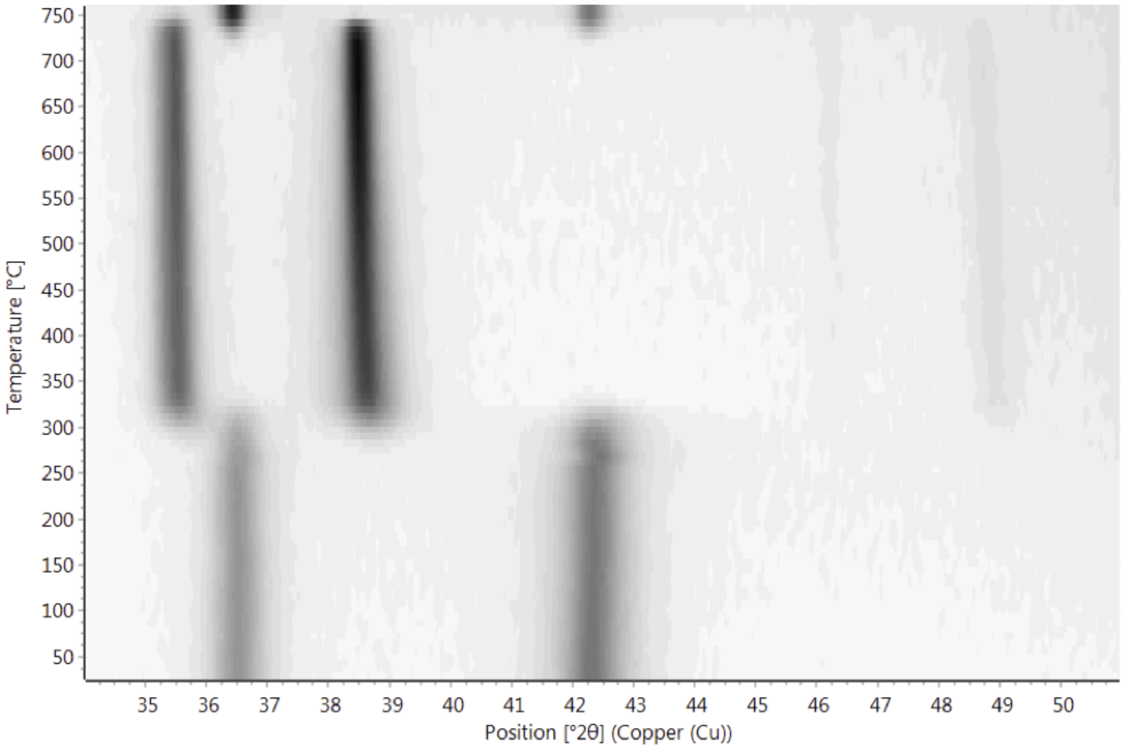


Figure S3: High-temperature GIXRD pattern of an ALD $Cu_2O$ film measured at 20 mbar N2 (flow 40 sccm). The $Cu_2O$ film with most intense reflections (111) at 36.4° and (200) at 42.3°, oxidises into CuO at 300 °C, as seen in appearance of CuO (002) and (111) reflections at $35.4^{circ}$ and 38.6°, respectively.

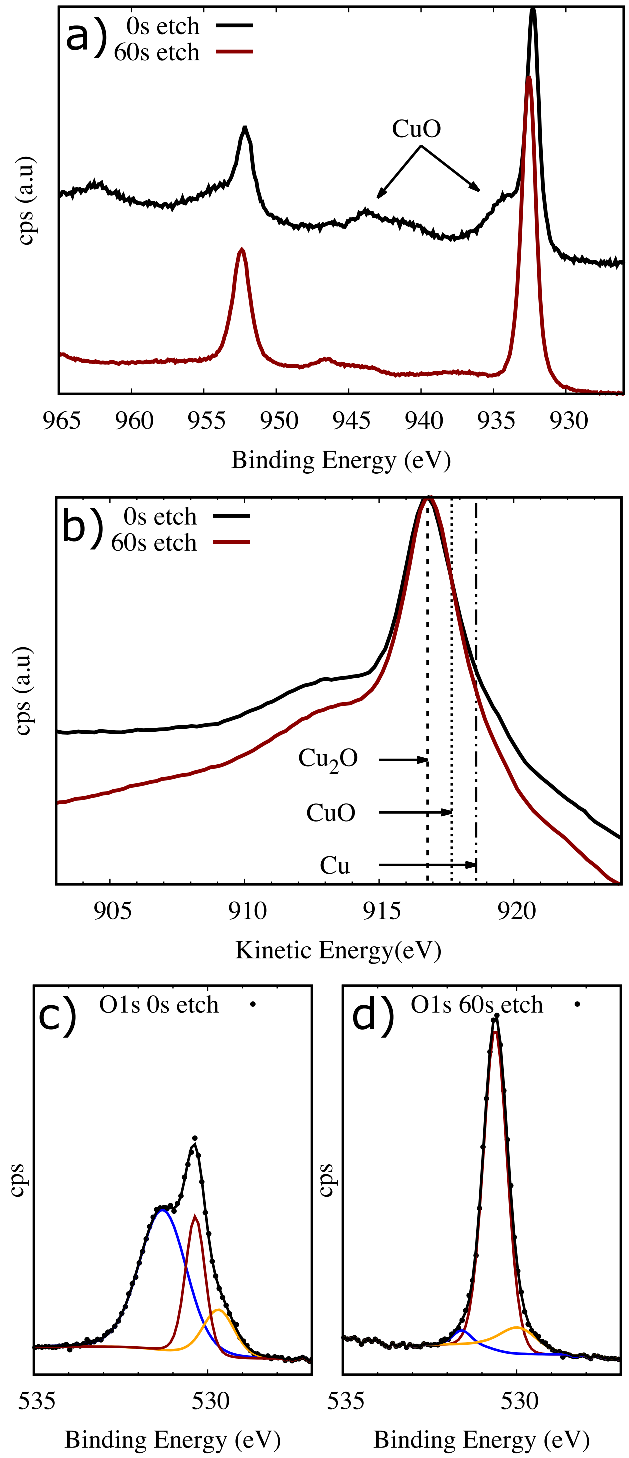


Figure S4: XPS spectra of the as deposited $Cu_2O$ film, (a) Cu 2p, (b) Cu LMM (normalized), (c)&(d) O1s, measured after 0 s and 60 s of 0.5 keV $Ar^+$ sputter surface cleaning. The deconvoluted peaks in (c) and (d) correspond to $Cu_2O$ lattice oxygen (dark-red), CuO (orange), and hydroxyl groups (-OH, blue)

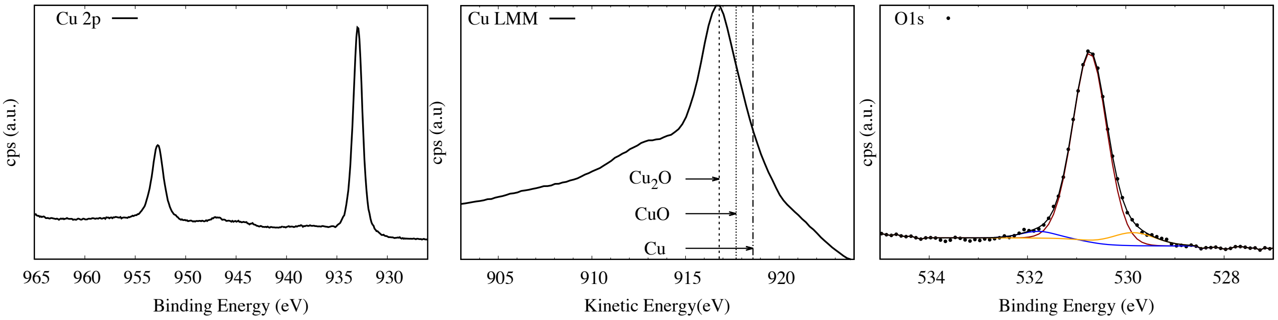


Figure S5: XPS Cu2p, Cu LMM, and O 1s spectra of the $Cu_2O$ film annealed 10 min in 1.5 mbar at 300 °C, measured after 30 s 0.5 keV $Ar^+$ sputter surface cleaning.

Table S1: Thermodynamics of oxidation reactions of $Cu^0$ into $Cu_2O$ and CuO by $H_2O$ or $O_2$

(a) $\mathbf{2Cu + H_2O(g) = Cu_2O + H_2(g)}$

| T (°C) | ΔH (kJ) | ΔS (J/K) | ΔG (kJ) |
|---|---|---|---|
| 0 | 73.003 | -32.630 | 81.916 |
| 100 | 73.969 | -29.640 | 85.030 |
| 200 | 75.132 | -26.886 | 87.853 |
| 300 | 76.389 | -24.477 | 90.419 |
| 400 | 77.705 | -22.363 | 92.758 |
| 500 | 79.054 | -20.494 | 94.899 |
| 600 | 80.417 | -18.837 | 96.864 |
| 700 | 81.766 | -17.374 | 98.673 |
| 800 | 83.071 | -16.097 | 100.345 |
| 900 | 84.288 | -15.011 | 101.899 |
| 1000 | 85.372 | -14.124 | 103.354 |

(b) $\mathbf{Cu + H_2O(g) = CuO + H_2(g)}$

| T (°C) | ΔH (kJ) | ΔS (J/K) | ΔG (kJ) |
|---|---|---|---|
| 0 | 84.200 | -49.639 | 97.759 |
| 100 | 85.596 | -45.317 | 102.506 |
| 200 | 87.210 | -41.489 | 106.841 |
| 300 | 88.896 | -38.257 | 110.823 |
| 400 | 90.599 | -35.519 | 114.508 |
| 500 | 92.287 | -33.180 | 117.940 |
| 600 | 93.941 | -31.169 | 121.155 |
| 700 | 95.540 | -29.434 | 124.183 |
| 800 | 97.064 | -27.942 | 127.050 |
| 900 | 98.490 | -26.671 | 129.779 |
| 1000 | 99.792 | -25.605 | 132.391 |

(c) $\mathbf{2Cu + O_2(g) = 2CuO}$

| T (°C) | ΔH (kJ) | ΔS (J/K) | ΔG (kJ) |
|---|---|---|---|
| 0 | -314.762 | -186.407 | -263.845 |
| 100 | -313.941 | -183.909 | -245.315 |
| 200 | -312.597 | -180.733 | -227.083 |
| 300 | -311.029 | -177.732 | -209.162 |
| 400 | -309.350 | -175.033 | -191.526 |
| 500 | -307.609 | -172.623 | -174.146 |
| 600 | -305.833 | -170.463 | -156.993 |
| 700 | -304.045 | -168.524 | -140.046 |
| 800 | -302.272 | -166.790 | -123.282 |
| 900 | -300.553 | -165.258 | -106.681 |
| 1000 | -298.933 | -163.932 | -90.223 |

(d) $\mathbf{4Cu + O_2(g) = 2Cu_2O}$

| T (°C) | ΔH (kJ) | ΔS (J/K) | ΔG (kJ) |
|---|---|---|---|
| 0 | -337.156 | -152.388 | -295.531 |
| 100 | -337.193 | -152.557 | -280.266 |
| 200 | -336.752 | -151.526 | -265.058 |
| 300 | -336.043 | -150.172 | -249.971 |
| 400 | -335.138 | -148.721 | -235.026 |
| 500 | -334.075 | -147.251 | -220.228 |
| 600 | -332.881 | -145.800 | -205.576 |
| 700 | -331.592 | -144.404 | -191.066 |
| 800 | -330.259 | -143.099 | -176.692 |
| 900 | -328.956 | -141.938 | -162.441 |
| 1000 | -327.773 | -140.969 | -148.298 |

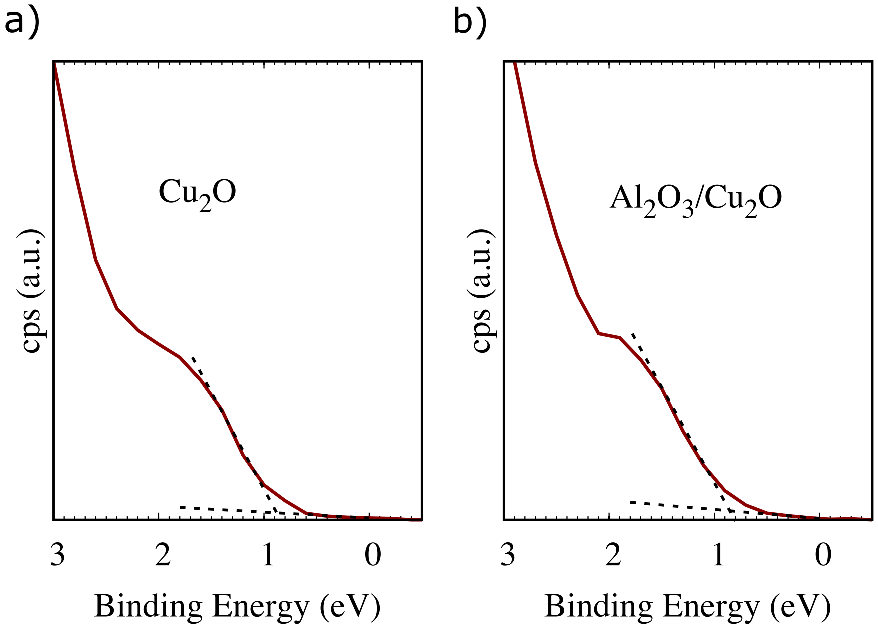


Figure S6: XPS valence edge spectra of a) $Cu_2O$ film ($E_F - E_{VB} = 0.9$ eV), and b) $Al_2O_3/Cu_2O$ interface after a 90 s sputtering with 0.5 keV $Ar^+$ ($E_F - E_{VB} = 0.9$ eV)

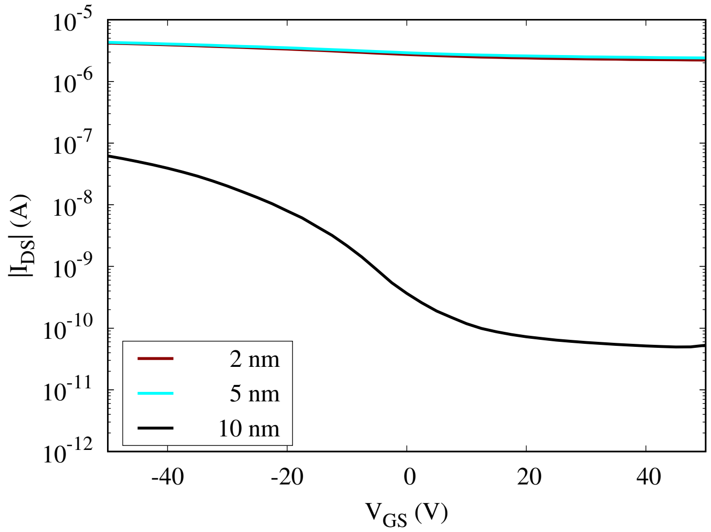


Figure S7: The effect of ALD $Al_2O_3$ layer thickness on the transfer characteristics of the $Cu_2O$ p-channel TFTs, all samples were annealed for 10 min at 300 °C 1.5 mbar $N_2$
